# Supplementary material for: An Iterated Az\'{e}ma-Yor Type Embedding for Finitely Many Marginals
Source: arXiv:1304.0368 source file (2014-01-06)
Supplement: Supplementary file 1 [file appendix_research.tex]

\newpage
 
\section{Ongoing Research}

\subsection{Sufficient Condition for Assumption \ref{ass:unicity_minimizers}}

Although Assumption \ref{ass:unicity_minimizers} was convenient in the construction and proof of our main result, it has the disadvantage that it is not very explicit. 

Let $(X_1,X_2)$ be a martingale with marginals $\nu_1$ and $\nu_2$.
\cite{RePEc:arx:papers:1304.2141} consider optimal lower bounds on $\E{\left| X_1 - X_2 \right|}$ of the form $\int g \dd \nu_1 + \int h \dd \nu_2$. 
For their construction they require some condition on the difference of the distribution functions of $\nu_1$ and $\nu_2$.
In our construction we have the additional state variable of the continuously sampled maximum and our construction depends on this variable. 
Hence, the fact that Assumption \ref{ass:unicity_minimizers} features quantities which relate to this variable should not surprise.

The following result provides a class of measures for which Assumption \ref{ass:unicity_minimizers} is satisfied.

\begin{Proposition}[Sufficient Condition]
\label{prop:sufficient_condition}
Let Assumption \ref{ass:unicity_minimizers}(i) holds and assume that $c_1,\dots,c_n$ are twice differentiable. % and that there exists an $x_{\star}>\sup\left\{ x: \mu_1((x,\infty)) = 1 \right\}$ such that
%\begin{align}
%b_1(x) < b_2(x) < \dots < b_n(x) \qquad \text{for all} \quad x \leq x_{\star}.
%\end{align}

Set $\mu_0 \equiv 0$ and $l_{\mu_n} := \sup\left\{ x: \mu_n((x,\infty)) = 1 \right\}$.
Suppose that for all $\alpha = \zeta_0 \leq \zeta_{1} \leq \dots \leq \zeta_{n} = \beta$, where either $\alpha>l_{\mu_n}$ or $\beta<r_{\mu_n}$, the measures 
\begin{align}
\lambda_1 := \restr{\mu_n}{[\alpha,\beta]} \qquad \text{and} \qquad 
\lambda_2 :=  \sum_{i=0}^{n-1} \restr{\mu_i}{[\zeta_{i}, \zeta_{i+1}]}
\label{eq:restriction_measures}
\end{align}
do not have the same mass or mean or are not in convex order.

Then $\mu_1,\dots,\mu_n$ satisfy Assumption \ref{ass:unicity_minimizers}(ii).
\end{Proposition}
\begin{proof}
The case $n=2$ follows from \cite[Section 3.5]{Brown98themaximum}.
For notational convenience we will only spell out the proof in the case $n=3$.
It should be clear that similar arguments apply for general $n \in \N$.

It follows immediately that 
\begin{align*}
c_i < c_{i+1} \qquad \text{for $i=1,\dots,n-1$.}
\end{align*} 

We will proceed by proving that if $\alpha < \beta$ are minimizers in \eqref{eq:suff_cond_unicity_minimzers} then 
\begin{align}
\restr{\lambda_1}{[\alpha,\beta]} \qquad \text{and} \qquad \lambda_2 =  \restr{\mu_1}{[\alpha,\xi_2]} + \restr{\mu_2}{[\xi_2,\beta]}
\end{align}
from \eqref{eq:restriction_measures} have the same mass and mean and are in convex order. 
This situation however is ruled out by our assumption.

We restrict to the following case,
\begin{align}
\imath_3(\beta;y)=2 \qquad \text{and} \qquad \imath_3(\alpha;y)=1.
\end{align}
The other cases follow similarly. 
 
Note that under our assumptions \eqref{eq:optimality_xi} holds for $\xi_3(y) = \alpha$ and $\xi_3(y) = \beta$.
 
\textit{Masses.}
The mass of $\lambda_1$ is $c'_3(\beta) - c'_3(\alpha)$.
The mass of $\lambda_2$ is
\begin{alignat*}{3}
& &&c'_2(\beta) - c'_2(\xi_2) + c'_1(\xi_2) - c'_1(\alpha) = \stackrel{\eqref{eq:optimality_xi}}{=} c'_2(\beta) + K_2(y) - K_1(y) - c'_1(\alpha) \\ &\stackrel{\eqref{eq:optimality_xi}}{=} &&  c'_3(\beta) - c'_3(\alpha)
\end{alignat*}
where for the last equality we applied \eqref{eq:optimality_xi} for $\alpha$ and $\beta$.

\textit{Means.}
The mean of $\lambda_1$ is
\begin{align*}
\int_{\alpha}^{\beta} x \mu_3(\dd x) = c_3(\alpha) - c_3(\beta) + (\beta- \alpha) c'_3(\beta) + \underbrace{\alpha \mu_3([\alpha,\beta])}_{\mathclap{=\xi_2 \mu_3([\alpha,\beta]) - (\xi_2-\alpha) (c'_3(\beta) - c'_3(\alpha))}}.
\end{align*}
The mean of $\lambda_2$ is
\begin{alignat*}{3}
&&&c_2(\xi_2) - c_2(\beta) + (\beta- \xi_2) c'_2(\beta) + \xi_2 \mu_2([\xi_2,\beta]) \\
&+&&  c_1(\alpha) - c_1(\xi_2) + (\xi_2- \alpha) \underbrace{c'_1(\xi_2)}_{\mathclap{=\mu_1([\alpha,\xi_2]) + c'_1(\alpha)}} + \alpha \mu_1([\alpha,\xi_2]).
\end{alignat*}
Observe that by optimality of $\alpha$ and $\beta$ and smoothness we have
\begin{align*}
\frac{\partial c^3}{\partial x}(\alpha,y) = \frac{c^3(\beta,y) - c^3(\alpha,y)}{\beta-\alpha} = \frac{\partial c^3}{\partial x}(\beta,y).
\end{align*}
Now we compute the difference of the means as
\begin{alignat*}{3}
&&&c^3(\alpha,y) - c^3(\beta,y) + (\xi_2-\alpha)\frac{\partial c^3}{\partial x}(\alpha,y) + (\beta-\xi_2)\frac{\partial c^3}{\partial x}(\beta,y)  \\
&-&& (y-\alpha)K_1(y) + (y-\beta)K_2(y)  \\
&-&& (\xi_2-\alpha)c'_3(\alpha) + (\xi_2-\alpha)K_1(y) - (\alpha - \xi_2)c'_3(\beta)  + (\beta-\xi_2)K_2(y) \\
&-&& c_2(\xi_2) + c_1(\xi_2) + \alpha \mu_3([\alpha,\beta]) - \xi_2 \mu_2([\xi_2,\beta]) - \xi_2 \mu_1([\alpha, \xi_2]) \\
=&&& (y-\xi_2)K_2(y) - (y-\xi_2) K_1(y) - c_2(\xi_2) + c_1(\xi_2) \\
&-&& (\xi_2-\alpha)c'_3(\alpha) - (\alpha - \xi_2)c'_3(\beta) - (\xi_2-\alpha)(c'_3(\beta) - c'_3(\alpha)) \\
&+&& \xi_2 \big(\mu_3([\alpha,\beta] - \mu_2([\xi_2,\beta]) - \mu_1([\alpha,\xi_2)) \big) \\
=&&&0
\end{alignat*}
by definition of $K_2(y)$ and the same mass of $\lambda_1$ and $\lambda_2$.

\textit{Convex Order.}
We have to show
\begin{align*}
\int (x-z)^+ \lambda_1(\dd x) \leq \int (x-z)^+ \lambda_2(\dd x) \qquad \text{for all $z \in [\alpha,\beta]$.}
\end{align*}

We compute for $z \in [\alpha,\beta]$ 
\begin{align*}
\int (x-z)^+ \lambda_1(\dd x) = c_3(z) - c_3(\beta) - (\beta-z) \underbrace{\mu_3([\beta,\infty])}_{\mathclap{=-c'_3(\beta)}}
\end{align*}
and for  $z \in [\alpha,\xi_2]$
\begin{alignat*}{3}
\int (x-z)^+ \lambda_2(\dd x) = & &&c_1(z) - c_1(\xi_2) - (\xi_2-z) \underbrace{\mu_1([\xi_2,\infty])}_{=-c'_1(\xi_2)} \\
								 &+&&c_2(\xi_2) - c_2(\beta) - (\beta - \xi_2) \underbrace{\mu_2([\beta,\infty])}_{=-c'_2(\beta)} + (\xi_2-z) \underbrace{\mu_2([\xi_2,\beta])}_{\mathclap{=c'_2(\beta) - c'_2(\xi_2)}}.
\end{alignat*}
For $z \in [\alpha,\xi_2]$, the difference of these two expression is
\begin{alignat*}{3}
&&&\overbrace{c^3(z,y) - c^3(\beta,y) + (\beta - z) ( c'_3(\beta) - c'_2(\beta) - K_2(y) ) }^{\geq 0} \\
&+&& (y-\beta) K_2(y) -(y-\xi_2)K_1(y) + (\beta - z) K_2(y) \\
&-&& c_2(\xi_2) + c_1(\xi_2) + (\xi_2-z) \underbrace{( c'_2(\xi_2) - c'_1(\xi_2))}_{\mathclap{=-K_2(y)+K_1(y)}} \geq 0
\end{alignat*}
by definition of $K_2(y)$.

The case $z \in [\xi_2,\beta]$ follows similarly.
\end{proof}

\subsubsection{Discussion of Necessity of Proposition \ref{prop:sufficient_condition}}

The conditions in Proposition \ref{prop:sufficient_condition} seem to exclude many measures for which our construction works.

For instance, one could construct two measures with the IMRV property which violate the assumptions of Proposition \ref{prop:sufficient_condition}.

\newpage

\subsection{Necessary and Sufficient Condition under Hobson Assumption}

\subsubsection{$n=2$}

\begin{Proposition}
\label{prop:charterization_n_2}
Let $n=2$ and assume that 
\begin{itemize} 
	\item[(a)] Assumption \ref{ass:unicity_minimizers}(i) holds,	
	\item[(b)] $ x \mapsto c_2(x) - c_1(x) $ is concave on $(x_l,x_r)$ and convex on $(-\infty,x_l]$ and $[x_r,\infty)$,
	\item[(c)] $c_1<c_2$,
	\item[(d)] $b_i$ is strictly increasing.
\end{itemize}

Then Assumption \ref{ass:unicity_minimizers}(ii) is equivalent to the following:
if $b^{-1}_2(y) < b^{-1}_1(y)$ then for all $\beta$ such that $ b_1^{-1}(y) \leq \beta <y$ we have
\begin{align}
\bar{\mu}_2^{\mathrm{HL}}(y) - \bar{\mu}_1^{\mathrm{HL}}(y) < \frac{c_2(\beta) - c_1(\beta)}{y-\beta}.
\label{eq:charterization_n_2}
\end{align}
\end{Proposition}
\begin{proof}
We prove necessity of \eqref{eq:charterization_n_2}. 
If we can find $y$ and $\beta$ such that 
\begin{align*}
\bar{\mu}_2^{\mathrm{HL}}(y) - \bar{\mu}_1^{\mathrm{HL}}(y) = \frac{c_2(\beta) - c_1(\beta)}{y-\beta}
\end{align*}
then we must also have
\begin{align*}
c'_2( b_2^{-1}(y) ) = c'_2(\beta) - c'_1(\beta) - \bar{\mu}_1^{\mathrm{HL}}(y).
\end{align*}
Together with
\begin{align*}
\frac{ c^2(b_2^{-1}(y),y)}{y - b_2^{-1}(y) } = \frac{c^2(\beta,y)}{y-\beta}
\end{align*}
this yields that Assumption \ref{ass:unicity_minimizers}(ii) is violated.

Now we prove sufficiency.
To this end, assume that Assumption \ref{ass:unicity_minimizers}(ii) is violated, i.e. there are $\alpha < \beta<y$ such that
\begin{align*}
\frac{ c^2(\alpha,y)}{y - \alpha } = \frac{c^2(\beta,y)}{y-\beta}
\end{align*}
and 
\begin{align}
\frac{\partial c^2}{\partial x}(\alpha,y) = \frac{\partial c^2}{\partial x}(\beta,y).
\label{eq:suff_proof_optimality_n_2}
\end{align}
We need to show that $\alpha = b_2^{-1}(y) < b_1^{-1}(y) \leq \beta$.

If $\alpha < b_1^{-1}(y)$ then by assumption $\alpha = b_2^{-1}(y)$. By \eqref{eq:suff_proof_optimality_n_2} and (b) it is not possible that $\alpha \geq b_1^{-1}(y)$ (there are two points where $c_2-c_1$ have the same slope but then at these points the second derivatives have different signs). Similarly, by \eqref{eq:suff_proof_optimality_n_2} and (d) it is not possible that $\beta < b_1^{-1}(y)$.
\end{proof}

Proposition \ref{prop:charterization_n_2} states that under the Hobson assumption (b) there can only be jumps of $\xi_2$ across $\xi_1$. 
We capture them by \eqref{eq:charterization_n_2}.

\subsubsection{$n=3$}

\newpage
\input{monotonicity_xi_tilde} 

%\newpage
%\input{refined_pathwise_inequality}
